# Supplementary material for: Representation Learning for Conversational Data using Discourse Mutual Information Maximization
Source: arXiv:2112.05787 source file (2022-05-03)
Supplement: Supplementary file 1 [file old-appendix.tex]

\section{Introduction}

Natural language text is a highly complex, structured random variable with variable length. Due to this, it is not possible to directly compute mutual information between two textual random variables. But in recent times, we have seen many fantastic neural model architectures for representing texts in a distributed semantic-vector space. These representations are mostly fixed length continuous vectors.

After this, our problem boils down to estimating mutual information between two continuous valued multivariate random variables (that is the continuous representation of texts in the aforementioned semantic vector space).

Hence, we call this estimate of mutual information between two textual random variables, representing two \textit{related} pieces of text, through their semantic-vector space representation as ``Semantic Mutual information'' or SMI.

\subsection{Computing SMI}
No computing mutual information between two continuous valued random variables is always a challenge by itself. But thankfully, in the last few years we have seen some very interesting methods for estimating mutual information between two continuous valued random variables.

\begin{enumerate}
 \item CPC
 \item DIMI-Estimator
 \item DIM
\end{enumerate}

We can use any of the estimators above to get an estimate of a semi between two texts.

\subsection{Difference from QA info Max:}

QAInfoMax does not obtain or estimate mutual information between to text but rather uses the D I am learning approach as a regularizer for its representation learning objectives. In this QA info Max paper, The MI computation is between two layers of representation learning network but for the same text only. It optimizes am I between Local and Global representation vectors.

Hence, our approach is novel in respect that we for the first time estimate and make use of MI between two related but distant pieces of text. No previous research has attempted in continuing or defining MI between texts. We are the first one to ever define mutual information between two textual random variables.

\textbf{Note:} Our method is not only limited to text but it is applicable to other domains or multi modal settings too, for example text and image or text and speech or text and classification label.


\section{Theory}
\subsection{Multi-View Learning}
Our work can be categorized in the general domain of representation learning through multi-view learning. \bs{federici ICLR 2020}. The main working principle of such \textbf{self-supervised learning} approaches is to maximize Mutual Information/similarity or minimize representation distance between two views of the same object.

\subsection{Multi-View Learning in NLP}
Under different nomenclature, we see application of this multi-view learning notion in NLP also. E.g. Next Sentence Prediction. We refrain from classifying CBOW, Skipgram or Masked-Language-Modeling into multi-view learning as these are generative model and their loss function is the error incurred in the generated output (reconstructed target).

Reconstruction can also be seen as a form of Mutual Information Maximization:
\begin{align}
 I(X;Y) = H_e(X) - H_e(X|Y) \geq H_e(X) - \mathcal{R}_{e,d}(X|Y)
\end{align}
where, $\mathcal{R}_{e,d}(X|Y)$ is the reconstruction error of $X$ given the representation $Y$.

The second line of approach that we also follow in this paper is based on the idea of learning a representation such that two different views of the same object when represented in this way will have high mutual information. We usually use various lower bounds to the actual MI as the loss function for optimization.

\begin{align}
 I(X;Y) \geq L(R_X;R_Y)
\end{align}

\subsection{Relation to Next Sentence Prediction, Conversational response Selection}

The task proposed in this paper for dialog representation learning using MI maximization is similar to NSP or CRS tasks. The main difference lies in the objective function used for learning each of these tasks. NSP and CRS usually uses cross-entropy loss with negative sampling as shown in the equation below.

\begin{align*}
 L=\sum_{c,r,r'}\left[-\log(g(c,r)) - \log(1-g(c,r'))\right]
\end{align*}

where, $(c,r)$ is the true context-response pair and $r'$ is a randomly selected negative sample based on some distribution over the utterances in the dataset.

In InfoMax learning, the loss functions that are used are provably a lower bound on the MI between the two views. There are various lower-bounds proposed over the years. For example,

\begin{align*}
 I_{InfoNCE} (X;Y) &= \mathbb{E}_{P} \left[ \log \frac{e^{f(x,y)}}{\mathbb{E}_{\tilde P} e^{f(x',y)}}\right]\\
 I_{JSD} (X;Y) &= \mathbb{E}_{P} [-sp(-T_{\phi, \omega}(x,y))] - \mathbb{E}_{P\times \tilde P} [sp(T_{\phi, \omega}(x',y))]
\end{align*}

$sp(.)$ is the softplus function. $sp(u) = \log(1+e^u)$. 

\section{Method}

\section{InfoNCE for Dialog}
\begin{align}
 f(c,r) &\propto \frac{p(r|c)}{p(r)}\\
 f(c,r) &= \exp(e_c^TWe_r)\\
 I(C,R) &\geq  \log (N) + \mathbb{E}_{P_{CR}} \left[ \log \frac{f(c,r)}{\sum_{r' \in R} f(c,r')} \right]
\end{align}


\begin{figure}
 \centering
 \includegraphics[width=\linewidth]{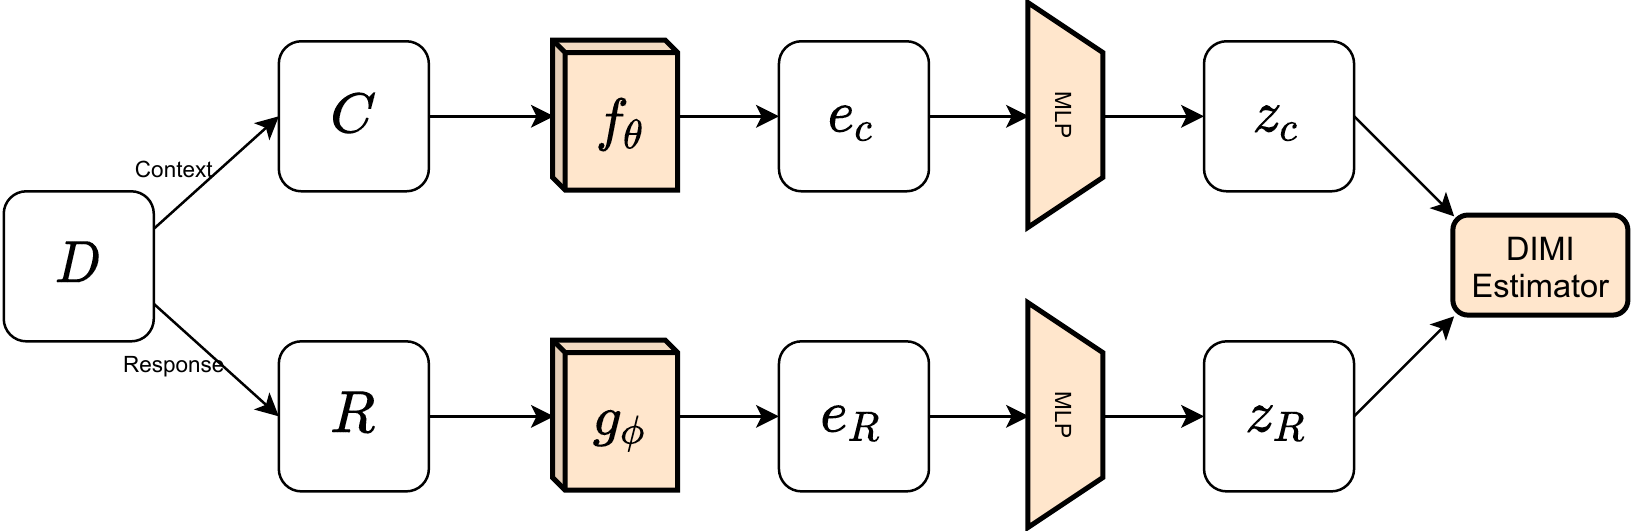}
 \caption{The overall SMI architecture}
\end{figure}

\section{Theory}

\textbf{Theorem:} SMI can really estimate the underlying MI between two pieces of text.

\textbf{Proof:} X, Y: front of variables representing the text will random variables and related to each other by some underlying phenomena
For example, dialogue, same source document, same event.

(Note that MI between X and Y maybe caused by different features or semantic effects depending on the task and domain)

The generation process of two such related random variables can be encapsulated by a generally graphical model as shown below:

In our proposed SMI approach, each of the two random variables are first independently and locally processed or encoded to some continuous representation space from which MI is estimated for those two continuous valued representations of X and Y, CRX and RY. We use any of the methods from literature for estimating MI.

1.the first inequality tells us that (the MI estimate obtained using the proposed method)) SMI will give us a lower bound on the true am I between the two textual random variables. 
2.also tells us that there is no trivial solution to the problem that we need to bother about.
3.If, RX or RY collapses to constant values, the entropy of these intermediate values variables will become zero.
If, the encoder can’t extract features in RX or or why that connects the samples of X and Y together, the mutual information will remain low as we are doing local processing The intermediate random variables cannot take the mutual information either.

This means that the EMI can only be increased by learning useful semantic features of X, Y in the representation RX, RY.

Hence, maximising SMI is a valid representation learning objective for textual data * for extracting task and domain specific features * on studies for learning generic NLP features * depending on the type of corpus. 


\begin{table*}[!htbp]
\begin{tabular}{@{}lR{1.2cm}R{1.6cm}rrR{1.6cm}rr@{}}
\toprule
                      & \multicolumn{1}{l}{} & \multicolumn{3}{c}{\textbf{SMI}} & \multicolumn{3}{c}{\textbf{Contrastive-SMI}} \\ \midrule
 &
  \multicolumn{1}{l}{} &
  \multicolumn{1}{l}{} &
  \multicolumn{2}{R{2.8cm}}{\textit{\textbf{Randomized Control (Marginal)}}} &
  \multicolumn{1}{l}{} &
  \multicolumn{2}{R{2.8cm}}{\textit{\textbf{Randomized Control (Marginal)}}} \\ \midrule
 &
  \textbf{Overall Quality} &
  \textbf{Observed Samples (Joint)} &
  \textbf{Mean} &
  \textbf{Conf. Interval} &
  \textbf{Observed Samples (Joint)} &
  \textbf{Mean} &
  \textbf{Conf. Interval} \\ \midrule
Original Ground-Truth & 4.3600               & 15.0814    & 5.0527   & ±3.798   & 21.3064        & 2.7244       & ±1.972       \\
Language Model        & 2.9800               & 5.3024     & 0.0093   & ±0.008   & 0.0061         & 2.3782       & ±1.003       \\
LSTM Seq2Seq          & 3.4700               & 7.6286     & 7.1450   & ±5.592   & 6.0091         & 3.4532       & ±2.387       \\
KV-MemNN              & 3.2500               & 14.1391    & 5.0077   & ±5.916   & 8.5948         & 1.8320       & ±0.891       \\
New Human Generated   & 4.8000               & 16.1917    & 4.1333   & ±3.361   & 37.7556        & 2.3592       & ±1.547       \\ \midrule
DailyDialog-Test & & 25.7786 & 0.6713& ±0.114 & 25.3283 & 1.4930 & ±0.380 \\ \bottomrule
\end{tabular}
\caption{Randomized Control Experiment}
\label{tab:random-control}
\end{table*}

\section{Experiments}
\subsection{Self-Supervised Pretraining} 
The first phase of learning in our approach is self-supervised pretraining with SMI maximization objective. We call this phase self-supervised as context-response pairs of dialog can be easily obtained without human annotators. Such sources include Reddit or Ubuntu IRC from which various dstc datasets were created in the past. 

Although to control for quality we use a mix of DailyDialog, Convai2, and Wizard-of-wikipedia datasets (train split) for our pretraining purposes. These sources contain conversations which are more human-like (avoids quirks on online chat/forums and contains less web-lingo), less noisy and avoids use of profanity language.

\subsection{MI as metric for dialog-system evaluation}


\subsection{pmi as metric for sample-level evaluation}

One may often want to measure the validity of a single context-response pair. But MI can be computed only at a distribution level (or batch/dataset level for empirical estimates). Depending on the loss function formulation for MI lower bound, we may be able to use an estimate of pointwise mutual information (pmi) for a single sample.

\paragraph{InfoNCE:} PMI can be computed for InfoNCE by normalizing the score of true $(c,r)$ pair by scores of a set of negative samples using softmax.

\begin{align*}
 pmi(c;r) = \log \frac{e^{f(c,r)}}{\sum_{r'} e^{f(c,r')}}
\end{align*}

Note that, $r'$ should be chosen from the same generative model's responses for other input contexts. This will be able to capture mode collapse / repetitive responses also as similar score values will be assigned to similar responses. So, SMI can account for such diversity issues also. \bs{NEED experimental VERIFICATION.}



\subsection{Toy-task for Model Validation}

\subsection{Downstream Task: SWDA Dialog-Act classification}

\subsection{InfoMax as a supervised learning objective for Ubuntu Response Selection}
\bs{SEPARATE PAPER}

\section{Preliminary Results}

\textbf{Completed Experiments and Initial Results:}
\begin{enumerate}
 \item Dialog Evaluation (system level): USR dataset
 \item Dialog Evaluation (sample level): USR dataset
 \item Downstream Task: SWDA
 \item Loss Functions: DIMI, InfoNCE
\end{enumerate}

% Please add the following required packages to your document preamble:
% \usepackage{booktabs}
\begin{table*}[!h]
\resizebox{\textwidth}{!}{%
\begin{tabular}{@{}lrrrrrrr@{}}
\toprule
 &
  {\textbf{Understand}} &
  {\textbf{Natural}} &
  {\textbf{Maintain Ctxt}} &
  {\textbf{Interesting}} &
  {\textbf{Use Knowledge}} &
  {\textbf{Overall Quality}} &
  {\textbf{Contrastive-SMI}} \\ \midrule
\textbf{Original Ground-Truth} & 0.99 & 2.89 & 2.82 & 2.67 & 0.56 & 4.36 & 21.306 \\
\textbf{Language Model}        & 0.97 & 2.63 & 2.02 & 2.24 & 0.08 & 2.98 & 0.006  \\
\textbf{LSTM Seq2Seq}          & 0.92 & 2.64 & 2.49 & 2.29 & 0.47 & 3.47 & 6.009  \\
\textbf{KV-MemNN}              & 0.93 & 2.7  & 2.18 & 2.56 & 0.17 & 3.25 & 8.595  \\
\textbf{New Human Generated}   & 1    & 2.97 & 2.88 & 2.87 & 0.96 & 4.8  & 37.756 \\ \bottomrule
\end{tabular}%
}
\caption{Comparision to other Quality Metrics}
\label{tab:compare-quality}
\end{table*}

% Please add the following required packages to your document preamble:
% \usepackage{booktabs}
\begin{table*}[!h]
\centering
\begin{tabular}{lrrr}
\toprule
\textbf{Model} & Mark & SWDA-Accuracy & Toy Task 1 \\ \midrule
VanillaTransformer* &  & \textbf{76.44} & \multicolumn{1}{l}{} \\
BERT-Linear/SE** &  & 67.14 & \multicolumn{1}{l}{} \\
SMI-Linear/DE & ? & \multicolumn{1}{l}{} & \multicolumn{1}{l}{} \\
SMI-Linear/SE & ? & \multicolumn{1}{l}{} & 0.7 \\
CSMI-Linear/DE & \#\# & 45.32 & 0.63 \\
CSMI-Linear/SE & \#\# & 49.58 & 0.64 \\
CSMI-Linear/SE & ? & 50.58 & 0.64 \\ \bottomrule
\end{tabular}
\caption{*All layers fine-tuned, other models fine tune with one-layer only, **(not fully trained, may reach upto 68), SE: shared encoder, DE: Dual Encoder, \#\#Pooler Ooutput, ?Last Hidden}
\label{tab:smi-finetune}
\end{table*}

\section{Related Works}
MI maximization has been highly prevalent in Computer Vision research community as an approach for self-supervised representation learning \cite{oord2018infonce,hjelm2018dim}. Although, the possibility of using this ``InfoMax principle'' as an optimization objective for representation learning has been proposed long back \cite{linsker1988}, it wasn't until recently that this was successfully applied for representation learning (using self-supervision). It was made possible by relatively recent discoveries of effective MI estimators for continuous valued random variables \cite{belghazi2018mine,song2019limitations,tschannen2019mutual}.

Here we would like to point out a crucial difference between self-supervised learning approaches of the vision domain and the one proposed here. In some (but not all) self-supervised image representation learning approaches, the two views are often augmented versions of the same portion of a source image. Hence, the actual content is of the image is still the same with some transformations applied to each. This is not the case is in our approach as the two views of the text are fully different in terms of surface form but are connected through a latent context.

\cite{oord2018infonce} first proposed the usage of InfoMax principle for semi-supervised representation learning. The estimatore used in this work falls within the generic family of estimators as proposed in a MINE. In the Deep Intomax paper, the authors showed an alternative learning approach wring the InfoMax principle. There instead of the multiview Mr maximization authors propose to apply InfoMax between global and local representations of an object ( image, text, etc. ).

Recently, Some recently published Recent works have also proposed solutions to different text-based tasks based on the InfoMax learning principle. In the GAInfoMan model, the authors applied the Deep Intoman / DIM loss as a regularizer to their problem and showed that it can help make the model learn more robust representation and avoid exploiting spurious correlations of data. Kong et al. show that many of the successful representation learning approaches used in NLP are well explained by the Intomax principle. As mentioned in the Theory section our method also has some similarities to the Next Sentence prediction task ( as seen in BERT, Skip thought ?. ... ) and the comversational response selection task. Although as shown in Section 2, our approach is more effective compared to NSP and Response Selection and avoids some potential limitations that arise in those settings. 

\section{Conclusion}

In this paper, we first proposed the concept of Semantic Mutual Information. Then we gove the theoretical base's for using SMI as an learning self-supervised learning objective. We showcase the working of this approach on various tasks around dialog and utterance representation learning. We further discussed how this approach is very suitable for learning domain / task targetted representations.


\section{Future Tasks: OpenIE Evaluation}

\bs{IMP:}

The SMI measure can be used for OpenIE evaluation also. With this we will be able to evaluate how much information is preserved.
